# Supplementary material for: Spatiotemporal plasma hologram
Source: arXiv:2505.12993 source file (2025-05-19)
Supplement: Supplementary file 1 [file Supplement_material_of_spatiotemporal_plasma_hologram.pdf]

# Supplement material of spatiotemporal plasma hologram

Zhaohui Wu,[1] Hao Peng,[2] Xiaoming Zeng,[3] Zhaoli Li,[3] Xiaodong Wang,[3] Xiao Wang,[3] Jie Mu,[3] Yanlei Zuo,[3] Kainan Zhou,[3] Nathaniel J. Fisch,[4] C. Riconda,[5] and S. Weber[6]

1) *National key laboratory of plasma physics, Research Center of Laser Fusion, China Academy of Engineering Physics, Mianyang, Sichuan,621900,China*

2) *Shenzhen Key Laboratory of Ultraintense Laser and Advanced Material Technology, Center for Advanced Material Diagnostic Technology, and College of Engineering Physics, Shenzhen Technology University,Shenzhen 518118, China*

3) *National key laboratory of plasma physics, Research Center of Laser Fusion, China Academy of Engineering Physics, Mianyang, Sichuan, 621900, China*

4) *Department of Astrophysical Sciences, Princeton University, Princeton, New Jersey 08540*

5) *LULI, Sorbonne Universit¨|, CNRS, ¨|cole Polytechnique, CEA, F-75005, Paris, France*

6) *ELI Beamlines facility, Extreme Light Infrastructure ERIC, 25241 Dolni Brezany, Czech Republic*

Keywords: plasma grating, laser compression, ultrashort laser pulse

## I. MO-PPT MODEL

For light-ionized plasma, the refractive index is given as

$$n = \sqrt{1 - n_e^2/n_c^2} \simeq n_e/2n_c = 1 + \rho P/2n_c \qquad (1)$$

where $\rho$ is the gas density, $P$ is the ionization potability per molecule, $I$ is the laser field. According to the molecular Perelomov-Popov-Terentév (MO-PPT) model the cycle-average ionization potability rat of a single molecule per unit time is given as

$$w = (\frac{3F}{\pi\kappa^3})^{1/2} \frac{B^2(m)A_m(\omega,\gamma)}{2^m m! \kappa^{2Z_c/\kappa-1}} (\frac{2\kappa}{F(1+\gamma^2)})^{2Z_c/\kappa-m-1} e^{\frac{-2\kappa^3 g(\gamma)}{3F}} \qquad (2)$$

where

$$g(\gamma) = \frac{3}{2\gamma}[(1+\frac{1}{\gamma^2})sinh^{-1}\gamma - \frac{\sqrt{1+\gamma^2}}{2\gamma}] \qquad (3)$$

where $\gamma = \sqrt{I_p/U_p} = \sqrt{2I_p}\omega/F$, $I_p$ is the ionization potential and $U_p$ the ponderomotive energy, $F$ is the electric field strength, $\omega$ is the laser frequency, $Z_c$ is the asymptotic charge, $\kappa = \sqrt{I_p/I_H}$, $\gamma$ is the Keldysh parameter. For a nonlinear molecule,

$$B(m) = \sum C_{lm} Q(l,m) \qquad (4)$$

and

$$Q(l,m) = (-1)^{(m+|m|)/2} \sqrt{\frac{(2l+1)(l+|m|)!}{2(l-|m|)!}} \qquad (5)$$

$A(\omega,\gamma)$ is given in the Ref.[1–3], and $C_{lm}$ can found in the Ref.[4]. For the plasma generated by the temporal-variation laser pulse, $P$ is given as

$$P = \int_0^\infty w dt \qquad (6)$$

By employing a 30 fs, 800 nm Gaussian laser pulse, we can calculate the ionization probability of both $N_2$ and $O_2$ by the MO-PPT model. The simulated ionization probability with the laser intensity form $10^{13}$W/cm$^2$ to $10^{15}$W/cm$^2$ are shown in Fig1. There are consistent with the theoretical and simulation result in Ref.[5–7].

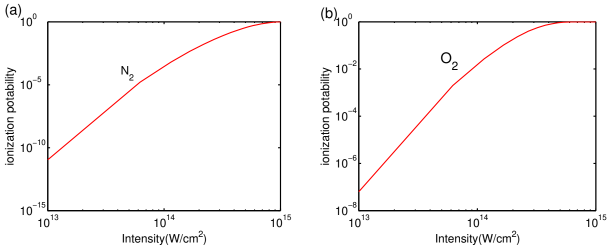


FIG. 1. Ionization portability of $N_2$ and $N_2$ with increasing laser intensity obtained by MO-PPT model.

By employing $I = I_0 + I_1 + 2\sqrt{I_0 I_1} cos(2\pi z/\Lambda)$ for the laser intensity and air (79% $N_2$, 21% $O_2$) for the background gas, $P$ can be estimated by the MO-PPT model. Then he effective refractive index $n_1$ is obtained from the first Fourier mode of $P$ . Finally, the diffractive intensity is calculated by $I \propto \rho^2 \Lambda \int_0^\Lambda Pe^{-j2\pi z/\Lambda} dz$. The simulation result shown in Fig2 indicates that the diffractive intensity is approximate linearly increasing with the object intensity with the laser intensity form $(0.5-4) \times 10^{14}$ W/cm$^2$. To confirm this, we measured the peak diffractive intensity with increasing object intensity in the experiment. The result matches well with the MO-PPT model as shown in Fig.2.

## II. EXPERIMENTAL SETUP

The experimental setup is shown in Fig.3. An initial laser picosecond laser pulse is provided by the Ti:shappire laser system, with a central wavelength of 800 nm and a bandwidth of 80 nm. The laser output was equally

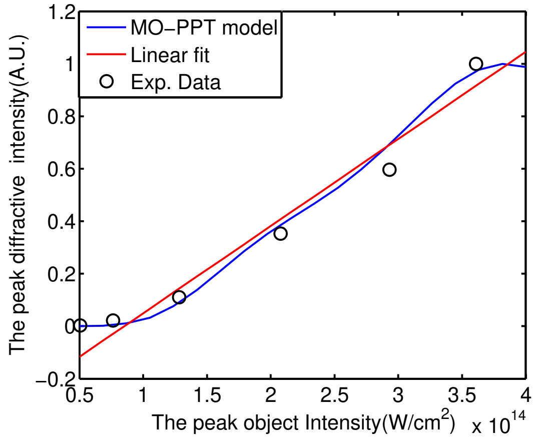


FIG. 2. Simulation and experimental peak signal with increasing object intensity.

split into two pulses by $BS_1$: one pulse, with an energy up to 6 mJ, was prolonged by a delay line of $M_3 - M_4$, and then directly focused into the air using an f/15 lens $L_1$ for the object pulse. It had a full width at half maximum (FWHM) focus diameter of $\sim 20$ $\mu$m and a FWHM duration of several picoseconds. The peak laser focused intensity is around $(3-4)\times 10^{14}$ W/cm$^2$ by adjusted the pulse energy and duration. The other pulse, used as the reference pulse, was first compressed to approximately 30 fs by a transmission grating pairs with groove of $300/mm$. It was also adjusted by the delay line of $M_5 - M_6$, and then cut off to a diameter of 1 mm by an aperture. As a result, it had an energy of 60 $\mu$J. It was then focused to the same region using an f/100 lens $L_2$, corresponding to a FWHM focused diameter $\sim 100\mu m$, and the focused intensity $2.5\times 10^{13}$ W/cm$^2$. As the reference pulse's focus size being five times larger than that of the object pulse, the beam was nearly uniform within the interference region, ensuring that the interference field only recorded information from the object pulse. Both pulses had an adjustable delay line to precisely synchronize their timing. The probe pulse was generated from the double frequency of the short reference pulse with a BBO crystal. It had a central wavelength of 420 nm and an FWHM spectral width of 10 nm. This pulse split by $BS_2$ was directed toward the plasma grating at a Bragg angle of approximately 60°. The intensity is kept below $10^{13}$ W/cm$^2$ in case of influencing the plasma grating. The first-order diffracted pulse was then collected using a lens and imaged to a CCD camera for further analysis.

## III. SUPPLEMENT EXPERIMENTAL RESULT

In order to test the spatial accuracy of the plasma hologram. We slightly tilted the angle of the phase plate to change the position of the ring structure in the objected

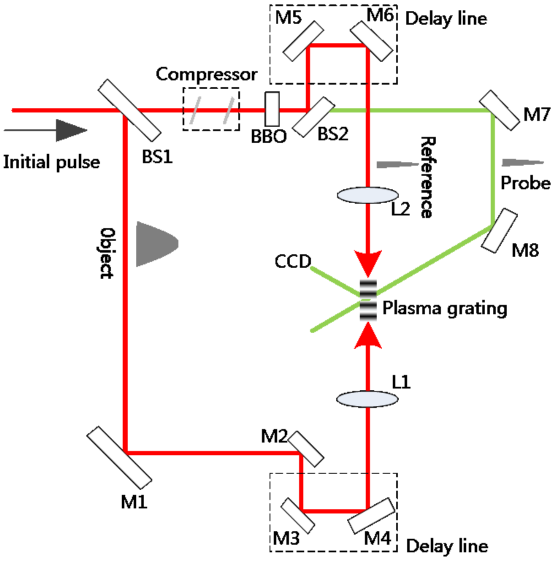


FIG. 3. Experimental setup for the spatiotemporal plasma hologram.

waist. As shown in Fig.4, the ring structure in the retrieved beam waist moved from left to right as the angle of phase plate was changed from −3°,0°,3°, implying the variation of the objected focus can be precisely captured by the volume plasma hologram.

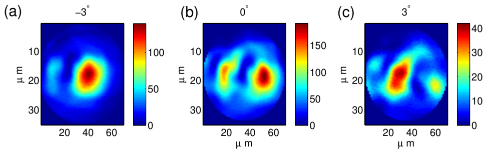


FIG. 4. Retrieved object focus with different tilt angle of the phase plate.

[1] F. A. Ilkov, J. E. Decker, and S. L. Chin, J. Phys. B: At Mol.Opt. Phys. **25**, 2005 (1992).
[2] Y. Z. Fu, S.-F. Zhao, , and X. X. Zhou, Chin. Phys. B **21**, 113101 (2012).
[3] A. M. Perelomov, V. S. Popov, and M. V. Terentèv, Sov. Phys. JETP **23**, 924 (1966).
[4] X. M. Tong, Z. X. Zhao, and C. D. Lin, Phys. Rev. A **66**, 033402 (2002).
[5] C. Guo, M. Li, J. P. Nibarger, and G. N. Gibson, Phys. Rev. A **58**, R4271 (1998).
[6] S.-F. Zhao, A.-T. Le, C. Jin, X. Wang, and C. D. Lin, Optics Communications **313**, 74 (2014).
[7] S.-F. Zhao, A.-T. Le, C. Jin, X. Wang, and C. D. Lin, Phys. Rev. A **93**, 023413 (2016).
